# Supplementary material for: A computationally lightweight safe learning algorithm
Source: arXiv:2309.03672 source file (2023-09-07)
Supplement: Supplementary file 1 [file appendix.tex]

\newpage
\onecolumn
\section*{Appendix}
\begin{proof}[Proof \textnormal{(}of Lemma \ref{lem:bounds}\textnormal{).}] We begin with the following simple observation
\begin{equation}
    \label{eqn:nadaraya-watson}
    \frac{\sum_{t=1}^n K_\lambda(a', a_t)\hat{h}_t(a,i)}{\sum_{t=1}^n K_\lambda(a', a_t)}\equiv\frac{\sum_{t=1}^n \frac{1}{c_K}K_\lambda(a', a_t)\hat{h}_t(a,i)}{\sum_{t=1}^n \frac{1}{c_K}K_\lambda(a', a_t)}.
\end{equation}
Clearly, $\frac{1}{c_K}K_\lambda(a', a_t)\leq 1$ Hence, without loss of generalization, in the sequel we assume that $K_\lambda$ is bounded by $1$.
Based on Assumption~\eqref{ass:observation_model}, we have, \cf~\cite{dean2021certainty},
\begin{equation}
\left| \sum_{t=1}^n\frac{K_\lambda(a', a_t)}{\kappa_n(a')}\hat{h}_t(a,i) - h(a',i) \right| \leq
\sum_{t=1}^{n}\theta _{t}\vert h( a_t,i) -h(
a',i) \vert +\left| \sum_{t=1}^{n}\theta _{t}\omega
_{t}\right|, \label{eq:uppbA}
\end{equation}%
where $\theta _{t}:= K_\lambda( a',a_t) /\kappa _{n}(a')$. Note that $\Sigma_{t=1}^n\theta _{t}=1$.
Due to Assumption $4$, if $K_\lambda( a',a_t) >0$, then $%
\lVert a'-a_t\rVert/\lambda\leq 1$. Therefore, (\cf~Assumption \eqref{ass:smoothness_assumption})%
\[
K_\lambda( a',a_t) >0\quad\Longrightarrow\quad \vert  h( a_t,i) -h(
a',i) \vert \leq L\lVert a'-a_t\rVert_{p} \leq L\lambda,
\]%
and since the weights $\theta _{t}$ sum up to $1$,%
\[
\sum_{t=1}^{n}\theta _{t}\vert h( a_t,i) -h(
a',i) \vert \leq Lh.
\]%
For the last term in (\ref{eq:uppbA}), observe that%
\begin{equation}\label{eq:transf}
\left| \sum\nolimits_{t=1}^{n}\theta _{t}\omega _{t}\right|
=\frac{1}{\frac{1}{c_K}\kappa _{n}(a')} \left| \sum\nolimits_{t=1}^{n}\frac{1}{c_K}K_\lambda( a',a_t) \omega _{t}\right|.
\end{equation}%
According to Lemma \ref{Lem:Tech_A}, the right-hand side of Eq.~\eqref{eq:transf} is upper bounded (with probability $1-\delta$) by
\[
\frac{1}{\frac{1}{c_K}\kappa_{n}(a')} \sigma \sqrt{2\log \left( \delta ^{-1}\sqrt{1+\sum
\nolimits_{t=1}^{n}\frac{1}{c_K^2}K_\lambda^{2}( a',a_t) }\right) \left(
1+\sum\nolimits_{t=1}^{n}\frac{1}{c_K^2}K_\lambda^{2}( a',a_t) \right) }.
\]
Furthermore, since $\frac{1}{c_K}K_\lambda( a',a_t) \leq 1$ (\cf~Assumption 4), we
obtain
\[
\frac{1}{\frac{1}{c_K}\kappa _{n}(a')} \left| \sum\nolimits_{t=1}^{n}\frac{1}{c_K}K_\lambda( a',a_t) \omega_{t}\right| \leq \sigma \sqrt{2\log
( \delta ^{-1}\sqrt{1+\frac{1}{c_K}\kappa_{n}(a')}) }\frac{\sqrt{1+\frac{1}{c_K}\kappa_{n}(a')%
}}{\frac{1}{c_K}\kappa _{n}(a')}.
\]%
Observe next that, if $\frac{1}{c_K}\kappa_{n}(a') > 1$, then%
\[
\frac{\sqrt{1+\frac{1}{c_K}\kappa _{n}(a')}}{\frac{1}{c_K}\kappa _{n}(a')}<\frac{\sqrt{2\frac{1}{c_K}\kappa _{n}(a')}}{%
\frac{1}{c_K}\kappa _{n}(a')}=\frac{\sqrt{2}}{\sqrt{\frac{1}{c_K}\kappa _{n}(a')}}.
\]%
Therefore, with probability $1-\delta$, for $\frac{1}{c_K}\kappa_{n}(a') > 1$ 
\begin{equation*}
\frac{1}{\frac{1}{c_K}\kappa _{n}(a')} \left| \sum\nolimits_{t=1}^{n}\frac{1}{c_K}K_\lambda( a',a_t) \omega _{t}\right| \leq \frac{2 \sigma}{\frac{1}{c_K}\kappa _{n}(a')} \sqrt{%
\frac{1}{c_K}\kappa _{n}(a') \log \left( \delta ^{-1}\sqrt{1+\frac{1}{c_K}\kappa _{n}(a')}\right)},    
\end{equation*}
whereas for $0<\frac{1}{c_K}\kappa _{n}\leq 1$,%
\begin{align*}
\frac{1}{\frac{1}{c_K}\kappa _{n}(a')} \left| \sum_{t=1}^{n}K_{\lambda}( a',a_t) \omega _{t}\right| &\leq
\frac{\sigma}{\frac{1}{c_K}\kappa_{n}(a')} \sqrt{2\log\left(\delta ^{-1}\sqrt{1+\frac{1}{c_K}\kappa_{n}(a')}\right) }\sqrt{1+\frac{1}{c_K}\kappa _{n}(a')}\\
&\leq \frac{2\sigma}{\frac{1}{c_K}\kappa_{n}(a')} \sqrt{\log ( \sqrt{2}/\delta)},
\end{align*}
which completes the proof.
\end{proof} 

The following two lemmas are small variations of Theorem $3$ and Lemma $1$ in \cite{abbasi:2011}, respectively.

\begin{lem}\label{Lem:Tech_A}
Let $\{ v_{t}\colon t\in\mathbb{N} \} $ be a bounded
stochastic process and $\{ \omega _{t}\colon t\in\mathbb{N} \} $ be a i.i.d. sub-Gaussian
stochastic process, \ie~there exists a $\sigma >0$ such that for any $\gamma \in \mathbb{R}$, and $t\in\mathbb{N}$,

\begin{equation}\label{subgauss}
\E\{ \exp ( \gamma \omega _{t}) \} \leq \exp \left( \frac{%
\gamma ^{2}\sigma ^{2}}{2}\right).
\end{equation}%
Let also%
\[
S_{n}:=\sum\nolimits_{t=1}^{n}v_{t}\omega _{t}\quad\textnormal{and}\quad V_{n}:=%
\sum\nolimits_{t=1}^{n}v_{t}^{2}.
\]%
Then, for any $n\in\mathbb{N}$ and $0<\delta <1$, with probability $1-\delta$,%
\begin{equation}
\vert S_{n}\vert \leq \sqrt{2\sigma ^{2}\log ( \delta ^{-1}%
\sqrt{1+V_{n}}) ( 1+V_{n}) }.
\end{equation}
\end{lem}
\begin{proof}
Without loss of generality, let $\sigma=1$. For any $\eta\in \mathbb{R}$ let
\[
w_n(\eta) :=\exp\left( \eta S_n - \frac{1}{2}\eta^2 V_{n}\right).
\]
From Lemma~\ref{Lem:Tech_B}, we note for any $\eta \in \mathbb{R}$ that $\E\{ w_{n}(\eta)\} \leq 1$. Let now $H$ be a $\mathcal{N}( 0,1)$ random variable, independent of all other variables. Clearly, $\E\{ w_{n}(H |H \} \leq 1$. Define%
\[
w_{n}:=\E\{ w_{n}( \eta ) |v_t,\omega_t \colon t\in\mathbb{N}\}.
\]%
Then $\E\{ w_{n}\} \leq 1$ since $\E\{ w_{n}\} =\E\{\E\{ w_{n}( H) |v_t, \omega_t\colon t\in\mathbb{N} \}\} = \E\{ w_{n}( H ) \} = \E\{ \E\{
w_{n}(H) |H \} \} \leq 1$. We can also express $w_n$ directly as
\begin{align*}
w_{n} &=\frac{1}{\sqrt{2\pi }}\int \exp\left( \eta S_{n}-\frac{1}{2}%
\eta ^{2}V_{n}\right) \exp\left( \frac{-\eta ^{2}}{2} \right) d\eta 
\\
&= \frac{1}{\sqrt{2\pi }}\int \exp\left( -\frac{1}{2}( V_{n}+1)
\eta ^{2}+S_{n}\eta\right) d\eta,
\end{align*}%
which further gives%
\begin{align*}
w_{n} &=\frac{1}{\sqrt{2\pi }}\int \exp\left( -\frac{1}{2}\frac{(
\eta -\frac{1}{1+V_{n}}S_{n}) ^{2}}{( 1+V_{n}) ^{-1}}\right) \exp\left( \frac{1}{2}\frac{S_{n}^{2}}{1+V_{n}}\right) d\eta  \\
&=\frac{1}{( 1+V_{n}) ^{1/2}}\exp\left( \frac{1}{2}\frac{%
S_{n}^{2}}{1+V_{n}} \right) \int \frac{1}{( 1+V_{n}) ^{-1/2}\sqrt{%
2\pi }} \exp\left( -\frac{1}{2}( \frac{\eta -\frac{1}{1+V_{n}}S_{n}}{%
( 1+V_{n}) ^{-1/2}}) ^{2}\right) d\eta  \\
&=\frac{1}{( 1+V_{n}) ^{1/2}} \exp\left( \frac{1}{2}\frac{%
S_{n}^{2}}{1+V_{n}}\right).
\end{align*}
Therefore $\mathbb{P}\{ \delta\, w_{n}\geq 1\} $ is equal to%
\begin{align*}
\mathbb{P}\left\{ \frac{\delta }{( 1+V_{n}) ^{1/2}}\exp\left( \frac{1}{2}%
\frac{S_{n}^{2}}{1+V_{n}}\right) \geq 1 \right\}
&= \mathbb{P}\left\{ \exp\left( \frac{1}{2}\frac{S_{n}^{2}}{1+V_{n}}\right) \geq ( 1+V_{n}) ^{1/2}%
\frac{1}{\delta } \right\} \\
&= \mathbb{P}\left\{ \frac{S_{n}^{2}}{1+V_{n}}\geq 2\log \left[ ( 1+V_{n})^{1/2}\frac{1}{\delta }\right] \right\} \\
&= \mathbb{P}\left\{ S_{n}^{2}\geq 2\log \left[ \frac{\sqrt{1+V_{n}}}{\delta }\right]
( 1+V_{n}) \right\}. 
\end{align*}
Recall now that $\E\{w_{n}\}\leq 1$. Hence, due to Markov's inequality,%
\[
\mathbb{P}\{ \delta\, w_n \geq 1\} \leq \delta\, \E\{ w_{n}\} \leq \delta,
\]%
which completes the proof.
\end{proof}

\begin{lem}\label{Lem:Tech_B}
Let $\{ v_{t}\colon t\in\mathbb{N} \} $ and $\{ \omega _{t}\colon t\in\mathbb{N} \} $ be as in Lemma \ref{Lem:Tech_A}. For any $\eta\in \mathbb{R}$, define%
\begin{equation}
w_{n}( \eta ) :=\exp \left( \sum_{t=1}^{n}\frac{\lambda \omega
_{t}v_{t}}{\sigma }-\frac{1}{2}\eta ^{2}v_{t}^{2}\right).
\end{equation}%
Then, $\E\{ w_{n}( \eta ) \} \leq 1$.
\end{lem}

\begin{proof}
Let
\[
D_t := \exp\left(\frac{\eta \omega _{t}v_{t}}{\sigma }-\frac{1}{2}\eta
^{2}v_{t}^{2}\right).
\]%
Clearly $w_{n}(\eta) = D_1 D_ 2 \dots D_n$. Note that
\begin{align*}
\E\{ D_t | v_t\} 
&= \E\left\{ \left. \exp\left( \frac{\eta\omega_t v_t}{\sigma}\right) / \exp\left( \frac{1}{2} v_t^2\eta^{2}\right) \right| v_t \right\} \\
&= \E\left\{ \left. \exp\left( \frac{\eta \omega_t v_t}{\sigma}\right) \right| v_t \right\} /\exp\left( \frac{1}{2} v_t^2\eta^2\right) 
\end{align*}
Hence, due to \eqref{subgauss}, 
\[
\E\{ D_t|v_t \}
\leq \exp\left[ \frac{( \eta v_t/\sigma )^2 \sigma^2}{2} \right] /\exp\left(\frac{1}{2} v_t^2\eta^2 \right)
= 1.
\]%
Next, for every $t\in\mathbb{N}$,%
\[
\E\{ w_n(\eta) |v_n \} = \E\{ D_1 \cdots D_{n-1} D_n | v_n \} = D_1 \cdots D_{n-1} \E\{ D_n|v_n \} \leq w_{n-1}(\eta) .
\]%
Therefore%
\begin{align*}
\E\{ w_{n}( \eta) \}
= \E\{ \E\{ w_{n}(\eta ) |v_{n}\} \}
\leq \E\{ w_{n-1}(\eta) \}
\leq \dots
\leq \E\{ w_1(\eta) \}
= \E\{ \E\{ D_1|v_1 \} \}
\leq 1,
\end{align*}
which completes the proof.
\end{proof}
